# Supplementary material for: Anatomy of triply-periodic network assemblies: Characterizing skeletal and inter-domain surface geometry of block copolymer gyroids
Source: arXiv:1801.03141 source file (2018-01-09)
Supplement: Supplementary file 1 [file Prasad_2018_SI.pdf]

# Electronic Supplementary Information for "Anatomy of triply-periodic network assemblies: Characterizing skeletal and inter-domain surface geometry of block copolymer gyroids"

Ishan Prasad
*Department of Chemical Engineering, University of Massachusetts, Amherst, Massachusetts 01003, USA*

Hiroshi Jinnai
*Institute of Multidisciplinary Research for Advanced Materials (IMRAM), Tohoku University, Katahira, Aoba-ku, Sendai, 980-8577, Japan*

Rong-Ming Ho
*Department of Chemical Engineering, National Tsing Hua University, Hsinchu 30013, Taiwan*

Edwin L. Thomas
*Department of Material Science and Nano Engineering, Rice University, Houston, TX 77005, USA*

Gregory M. Grason
*Department of Polymer Science and Engineering, University of Massachusetts, Amherst, MA 01003, USA*

## S1. INTENSITY PATTERNS ALONG SYMMETRY DIRECTIONS FROM SCF PREDICTIONS AND EMT RECONSTRUCTIONS

The supplementary videos listed below show polymer block intensity patterns in as viewed in 2D slices transversing normal to three symmetry directions of both SCF (theory) and EMT (experimental) cubic DG assemblies, namely, $\langle 100\rangle$, $\langle 110\rangle$, $\langle 111\rangle$.

**List of supplementary videos**:
Supplemental Video 1. SCF data along $\langle 100\rangle$: *scf100.avi*
Supplemental Video 2. SCF data along $\langle 110\rangle$: *scf110.avi*
Supplemental Video 3. SCF data along $\langle 111\rangle$: *scf111.avi*
Supplemental Video 4. EMT data along $\langle 100\rangle$: *emt100.avi*
Supplemental Video 5. EMT data along $\langle 110\rangle$: *emt110.avi*
Supplemental Video 6. EMT data along $\langle 111\rangle$: *emt110.avi*

## S2. COMPARISON OF "+"/"-" GRAPH FITS FOR BOTH SINGLE GYROID DOMAINS

As described in Section 2.2 of the main text, each tubular SG network domain (labelled as 1 and 2 for clarity) is fit with pre-aligned (10,3)-a nets of both "+" and "-" chirality. In Fig S2, we compare the fits of opposing graphs to the same tubular network domain, for both domains. The polar histogram shows all dihedral angles of the extracted skeletal graph while the solid (red/blue) line represents the predicted value of their corresponding ideal (10,3)-a graphs. The mean value of the network chirality order parameter, $\langle \chi_{2\theta}^{s,g}\rangle$ and its standard deviation, $\sigma_{2\theta}^{s,g}$ quantify the goodness of fit and determine the correct graph-domain fit, here $s$ is the "+"/"-" (10,3)-a graph and $g = 1$ or 2 is the index of the tubular SG domain. As in the main text, we analyze only the dihedral angles corresponding to internal edges of the clipped graphs (i.e., with no vertices at the boundary of the 3D volume). The local chirality, $\chi_{2\theta}$, histogram shows the distribution for dihedral angle of each triplet of consecutive graph edges. We find that in Fig. S1 A ("-" graph to domain 1) and 1 B ("+" graph to domain 2), the mean chirality of extracted graphs match the sign of dihedral rotations of their corresponding ideal graphs and that the standard deviation of each distribution ($\approx$ 0.5) is smaller than the difference between the mean values of the "+" and "-" graphs ($\approx$ 0.73). Whereas, in Fig. S1 C ("-" graph to domain 2) and 1 D ("+" graph to domain 1), the mean chirality values are negligible in compared to the standard deviation ($\approx$ 0.7) of the $\chi_{2\theta}$. Despite the inherent statistical variations of chirality shown in Fig. S1 A and B, comparison to random dihedrals from "wrong" handedness (10,3)a fits in Fig. S1 C and D illustrate ability of the graph analysis to identify proper chirality (as measured by sense of dihedral rotations) of SG tubular subdomains of reconstructed DG assemblies..

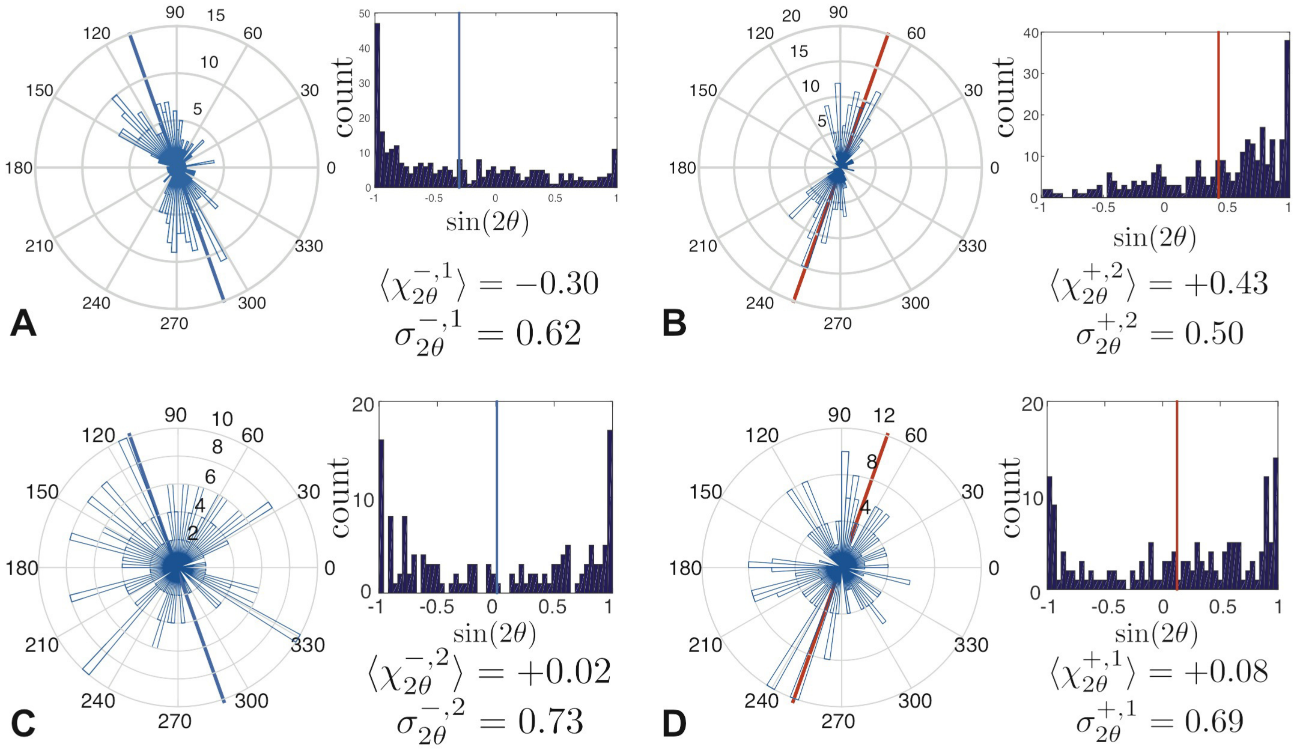


Figure S1: Comparison between "+"/"-" graph fits to each tubular network domain. (A) "-" graph to domain 1, (B) "+" graph to domain 2 (C) "-" graph to domain 2 (D) "+" graph to domain 1.

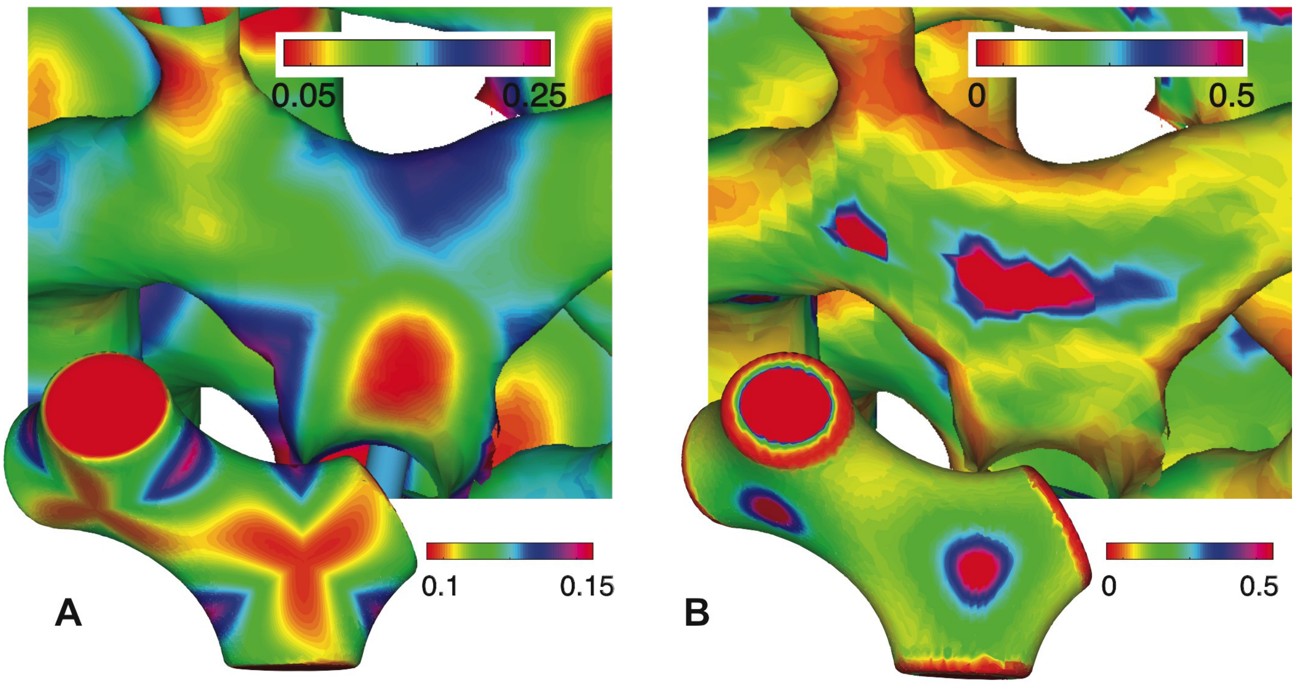


Figure S2: Domain thickness measures from EMT reconstructions with the corresponding ideal two-node strut from SCF theory. (A) $L_{\mathrm{i-g}}/D$. (B) $L_{\mathrm{focal}}/D$. Note that in (A) the different color scales are chosen to better highlight the relative local surface-skeleton distances in distinct regions of the IMDS for both SCF and EMT reconstructions.

## S3. DOMAIN THICKNESS MEASURES, $L_{\text{focal}}$ AND $L_{\text{i-g}}$, FROM EMT RECONSTRUCTIONS

In Section 3.2, we analyzed three local measures of domain thickness, the focal distance, $L_{\text{focal}}$, based on local curvature of the IMDS, and two measures of skeleton to surface distances. Fig 7 A and 7 E of the main text show the distribution of surface-to-skeleton, $L_{\text{i-g}}$ and focal, $F_{\text{focal}}$, distances on the IMDS of the ideal two-node strut obtained from SCF theory. In Fig S2, we show similar perspectives obtained from the EMT reconstructions of experimental SIS double gyroid morphology, showing relatively smaller and larger values of $L_{\text{i-g}}$ and $L_{\text{focal}}$ respectively in the "flatter" regions of the IDMS approximately tangent to the plane of the 3-fold junctions.
